# Supplementary material for: Two-dimensional inference of divertor plasma characteristics: advancements to a multi-instrument Bayesian analysis system
Source: arXiv:2403.12819 source file (2024-10-25)
Supplement: Supplementary file 1 [file AppendixOld.tex]

\begin{appendices}
\section{Prior Probability Distributions}
An example fit for the argument of Table \ref{tab:grid-enabled priors} is shown in Figure. This was representative of all priors specified in (). The majority of prior arguments, as expected lie at low values. However a maximum-likelihood fit to the data using a normal distribution finds that the steep tails under-fit the high prior argument values. This is more easily accommodated in 

\begin{figure}
    \centering
    \includegraphics[width=\linewidth]{Figures/Prior Histogram.png}
    \caption{Prior Histogram}
    \label{fig:prior_hist}
\end{figure}

\section{Optimisation}
For adequate mesh resolution, 744 vertices were used. For the inference, Te, ne, n0, He0, He1 and Qmol are required at each vertex. This results in sampling space of 4464 dimensions. For convergence on the MAP, a gradient ascent algorithm was used. Owing to such a high dimensional parameter space, stochastic gradient descent was costly and so the analytic gradient for the posterior was provided. This restricted the available priors to those that had an analytic gradient. 

Since the posterior distribution could not be guaranteed to be smooth, a hybrid approach of first order and second order optimisation methods was used. The second order L-BFGS optimiser () method quickly found local posterior probability peaks. The momentum-based, first order adam optimiser () managed to better circumvent local maxima and better navigate the non-smooth space. Further a range of `learning rates' were deployed to (). These hybrid approaches were wrapped into a generational algorithm whereby ().

The Cauchy distribution chosen for the priors resulted in slower convergence owing to the increasingly shallow gradient in log-probability space shown in Figure~\ref{fig:prior_hist}. To aid this slow convergence, the generational algorithm was chosen to begin using a posterior comprised of Normal distributions before switching to the Cauchy distribution for the remainder of the optimisation. This was found to ().

\section{Sampling}
Hamiltonian Monte Carlo (HMC) was used for sampling of the posterior distribution owing to its ability to handle high dimensional problems (). HMC has two variables that significantly impact its performance: the time step used in the `Leap Frog' integration, $\varepsilon$, and the number of Leap Frog steps, $L$. Following (Neal), the time step was chosen as the square root of the smallest eigenvalue of the covariance matrix of our parameters (which was estimated by calculating the Hessian in the vicinity of our MAP result and equating this to the inverse covariance). $\varepsilon$ was found to be $10^{-3}$ which promoted an issue: as (Neal) mentions, the benefits of HMC are fully realised when $\varepsilon L$ are large enough such that the particle reaches a U-Turn point. We include in our analysis parameters for which we hold very little information and so the ball would be expected to be fully cover the space before a U-turn is found. These, expected to have the largest covariance, can be used to identify a reasonable value for L. This distance travelled in a flat dimension is,
\begin{equation}
    s = pM^{-1} L \varepsilon
\end{equation}
Since $p\sim(N(0, M)$, we use the expectation value for a normal distribution of $\sqrt{2/\pi}$ and, for ease, assume a diagonal mass such that 
\begin{equation}
    s_{max} \sim \sqrt{\frac{2}{\pi}}\sigma_{max} L \sigma_{min}
\end{equation}
Rearranging,
\begin{equation}
    L \sim s_{max}\sqrt{\frac{\pi}{2}}\frac{1}{\sigma_{min}\sigma_{max}}
\end{equation}


To cover such distance, L must be $\sim 10^6$, equating to roughly one day per step. For comprehensive samples, we desire each chain to run for minimally the number of dimensions in the problem (4500). To avoid such time consuming sampling procedures, we ran our sampling on a \textit{higher temperature} posterior distribution
\begin{equation}
    \log(\Tilde{P})= T \log(P).
\end{equation}
This higher temperature has the effect of scaling the Hessian, and in turn the number of steps by the reciprocal of the temperature. 
To return the samples from $\Tilde{f}$ to the original temperature $f$, we fit a Gaussian Kernel Density estimate to $\Tilde{f}$, scaled this pdf by $^{1./T}$ and performed acceptance/rejection sampling on the $\Tilde{f}$ samples such that ,
\begin{equation}
    accept/reject \alpha < \Tilde{f} / f
\end{equation}

For this to be effective, we desire 45 00 

\end{appendices}
